# Supplementary material for: Spatiotemporal Modeling Encounters 3D Medical Image Analysis: Slice-Shift UNet with Multi-View Fusion
Source: arXiv:2307.12853 source file (2023-07-25)
Supplement: Supplementary file 1 [file _supplementary.tex]

\input{_constants}
\review % \review OR \cameraready

\documentclass[10pt,twocolumn,letterpaper]{article}
\input{cvpr_header}
\myexternaldocument{_main}
\begin{document}
%% TITLE
\title{\paperTitle \\ Supplemental Material}
\author{\authorBlock}
\maketitle

\input{12_appendix}

{\small
\bibliographystyle{ieee_fullname}
\bibliography{11_references}
}

\end{document}
